# Supplementary material for: WOMD-LiDAR: Raw Sensor Dataset Benchmark for Motion Forecasting
Source: arXiv:2304.03834 source file (2024-02-18)
Supplement: Supplementary file 1 [file supp_tab_test_set.tex]

\begin{table*}[b]
\begin{center}
\small
\begin{tabular}{@{}cc|ccc|ccc|ccc@{}}
\toprule
\multirow{2}{*}{Set} &
  \multirow{2}{*}{Model} &
  \multicolumn{3}{c|}{Vehicle} &
  \multicolumn{3}{c|}{Pedestrian} &
  \multicolumn{3}{c}{Cyclist} \\
 &
  &
  minADE $\downarrow$ &
  MR $\downarrow$ &
  mAP $\uparrow$ &
  minADE $\downarrow$ &
  MR $\downarrow$ &
  mAP $\uparrow$ &
  minADE $\downarrow$ &
  MR $\downarrow$ &
  mAP $\uparrow$ \\ \midrule
% \multicolumn{1}{l}{} &
%   LSTM~\cite{ettinger2021large} &
%   \multicolumn{1}{c}{1.34} & 
%   \multicolumn{1}{c}{0.25} & 
%   \multicolumn{1}{c|}{0.23} & 
%   \multicolumn{1}{c}{0.63} &
%   \multicolumn{1}{c}{0.13} &
%   \multicolumn{1}{c|}{0.23} &
%   \multicolumn{1}{c}{1.26} &
%   \multicolumn{1}{c}{0.29} &
%   \multicolumn{1}{c}{0.21} \\ \cmidrule(l){2-11} 
% \begin{tabular}[c]{@{}c@{}}Standard\\ Validation\end{tabular} &
%   Wayformer~\cite{nayakanti2022wayformer}
%   & 1.10
%   & 0.18
%   & 0.35
%   & 0.54
%   & 0.11
%   & 0.35
%   & 1.08
%   & 0.22
%   & \textbf{0.29}
%   \\ \cmidrule(l){2-11} 
%  &
%   \begin{tabular}[c]{@{}c@{}}Wayformer\\ + LiDAR\end{tabular} 
%   & \textbf{1.09}
%   & \textbf{0.17}
%   & \textbf{0.37}
%   & \textbf{0.54}
%   & \textbf{0.10}
%   & \textbf{0.37}
%   & \textbf{1.06}
%   & \textbf{0.21}
%   & 0.28
%   \\ 
% \midrule \midrule
\multicolumn{1}{l}{} &
  LSTM~\cite{ettinger2021large} &
  \multicolumn{1}{c}{1.34} & 
  \multicolumn{1}{c}{0.24} & 
  \multicolumn{1}{c|}{0.24} & 
  \multicolumn{1}{c}{0.64} &
  \multicolumn{1}{c}{0.13} &
  \multicolumn{1}{c|}{0.22} &
  \multicolumn{1}{c}{1.29} &
  \multicolumn{1}{c}{0.28} &
  \multicolumn{1}{c}{0.20} \\ \cmidrule(l){2-11} 
\begin{tabular}[c]{@{}c@{}}Standard\\ Test\end{tabular} &
  Wayformer~\cite{nayakanti2022wayformer}
  & 1.07
  & 0.17
  & 0.37
  & 0.54
  & 0.10
  & 0.37
  & 1.06 
  & 0.20
  & 0.30
  \\ \cmidrule(l){2-11} 
 &
  \begin{tabular}[c]{@{}c@{}}Wayformer\\ + LiDAR\end{tabular} 
  & 
  & 
  & 
  & 
  &
  &
  &
  &
  &
   \\ \bottomrule
\end{tabular}
\end{center}
\caption{\txbu{Marginal} \textbf{metrics on the} \txbu{standard} \textbf{validation set}. All metrics computed at 8s. We implement and compare our own WOMD~\cite{ettinger2021large} baseline, {\wf}~\cite{nayakanti2022wayformer} and {\wf} trained with {\lidar} data on the {\dbname} standard motion forecasting track.
}
\label{tab:supp_exp_res_standard}
\end{table*}
